# Supplementary material for: Exploring complex pattern formation with convolutional neural networks
Source: arXiv:2110.07306 source file (2021-10-14)
Supplement: Supplementary file 1 [file Supplementary_Information.pdf]

# Exploring complex pattern formation with convolutional neural networks
## - Supplementary information -

Christian Scholz* and Sandy Scholz
*Institut für Theoretische Physik II: Weiche Materie,*
*Heinrich-Heine-Universität Düsseldorf, 40225 Düsseldorf, Germany*

(Dated: October 13, 2021)

* christian.scholz@hhu.de

## I. ILLUSTRATION OF CLASSES IN THE GRAY-SCOTT MODEL

Classes previously identified in the literature for the Gray-Scott reaction diffusion model in two dimensions are ($\alpha$) Strong time-dependence, short spirals constantly form, collide and annihilate. ($\beta$) Strong time-dependent, chaotic oscillations. ($\gamma$) Stripes with some spontaneously oscillating regions. ($\delta$) Well-defined dots with local hexagonal order and many defects. ($\epsilon$) Pulsating dots that constantly appear and annihilate. ($\zeta$) Low concentration dots that are locally ordered with some defects that spontaneously appear. ($\eta$) Mixture of low value stripes and dots. ($\theta$) Stripe pattern with some dots, and no time-dependence as in $\gamma$. ($\iota$) Dots with short range or no order. ($\kappa$) Stable high concentration stripes that are strongly connected. ($\lambda$) Stable low concentration dots. ($\mu$) Simple snake-like stripes that hardly connect. ($\nu$) Frequent, mostly stable local defects that slightly repel. ($L$) Homogeneous low concentration. ($H$) Homogeneous high concentration. A representative pattern of each class after a simulation time of $t = 15000$ is shown in Fig. S1. Animations of the full simulations are shown in supplementary movie 1.

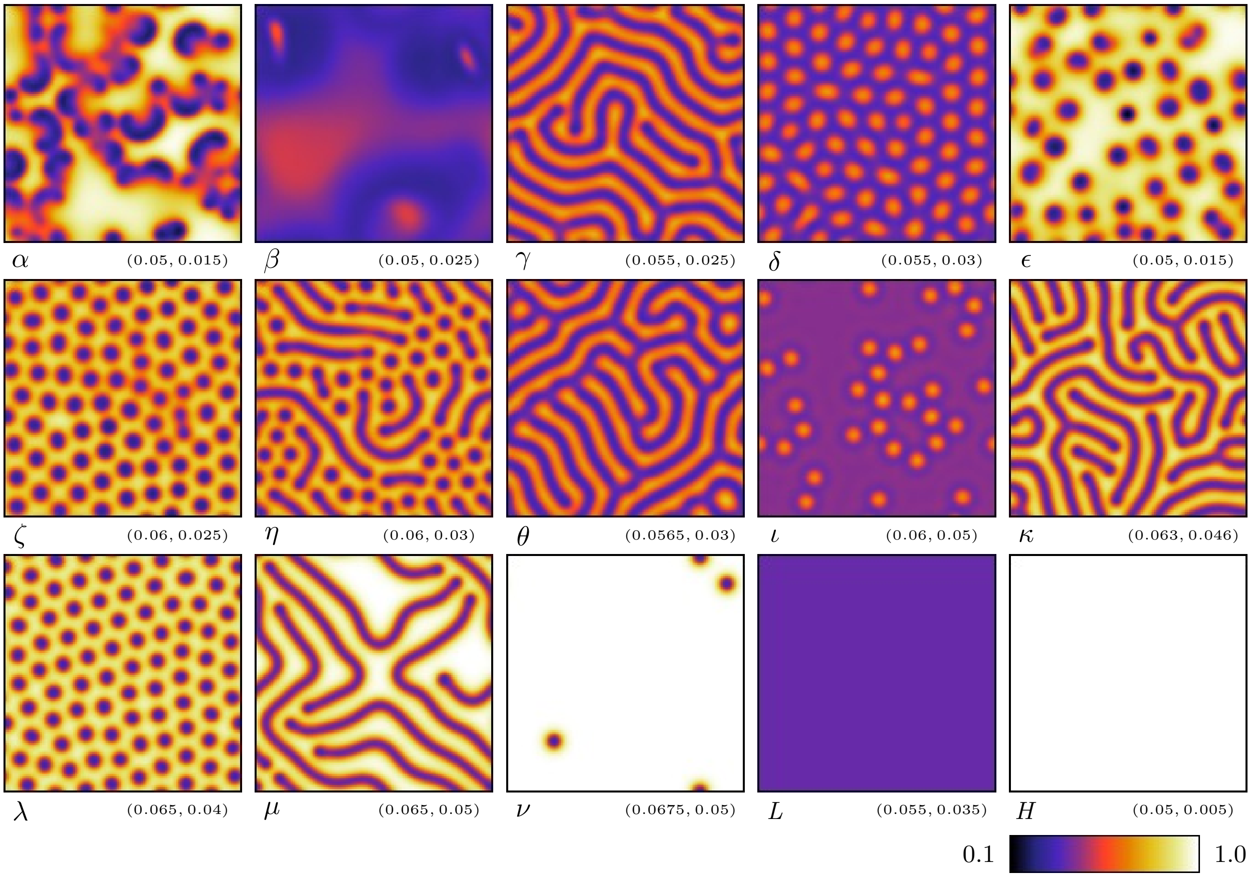


FIG. S1. Typical classes of homogeneous, heterogeneous and spatio-temporal patterns in the Gray-Scott model. The patterns are obtained on a grid of $128^2$ units at $t = 15000$ with $D_u = 0.2$ and $D_v = 0.1$. Reaction rate values are displayed below each pattern in the format $(k, f)$.

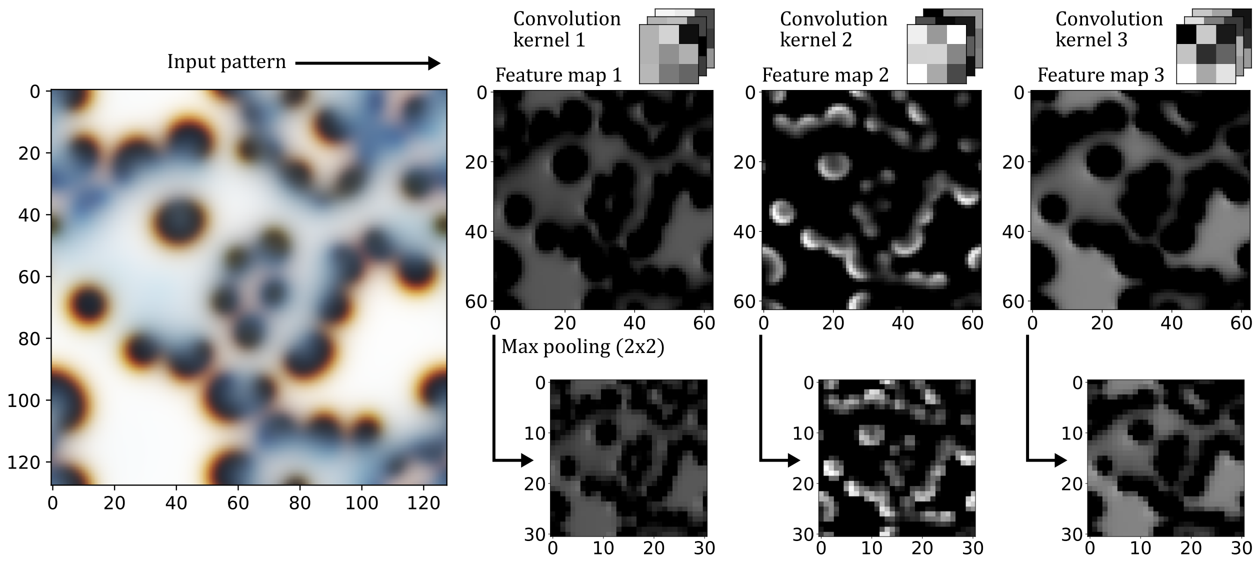


FIG. S2. Examples of three feature maps (out of 32) for the first convolution layer (i.e. application of convolution operation and relu activation function) in our model to an input pattern from class $\alpha$ and application of 2D max pooling.

## II. ILLUSTRATION OF CONVOLUTION AND MAX POOLING ON EXAMPLE IMAGES

In this section we demonstrate how to extract and display convolution kernels from a layer in the CNN, feature maps for a specific input pattern and the result of a max pooling operation on the feature maps. The following minimal code example can be used to display the above properties:

```
# Load dependencies
import matplotlib.pyplot as plt
import tensorflow as tf
import numpy as np
import pickle


# Load the required data and model
dataset_train = np.array(pickle.load(open("Dataset_2D_train.p", "rb")))
data = dataset_train[:50] # pick out the alpha patterns
del dataset_train
```

```
model = tf.keras.models.load_model("model_CNN_2D")

# Extract first convolution layer
filters, biases = model.layers[1].get_weights()

# Display kernels for first three feature maps
for iFilters in range(3):
    vmin = np.min(filters[:,:,0:3,iFilters])
    vmax = np.max(filters[:,:,0:3,iFilters])
    plt.figure()
    plt.imshow(filters[:,:,0,iFilters], vmin =vmin, vmax=vmax,cmap = 'gray')
    plt.xticks([])
    plt.yticks([])

# Extract and display first three feature maps
extractor = tf.keras.Model(inputs=model.inputs,
                        outputs=[layer.output for layer in model.layers])
features = extractor(data)

vmin = np.min(features[1][0,:,:,0:3])
vmax = np.max(features[1][0,:,:,0:3])
for iFeatures in range(3):
    plt.figure()
    plt.imshow(features[1][0,:,:,iFeatures], vmin =0, vmax=vmax, cmap = 'gray')

# Display first three feature maps after 2x2 max pooling
feature_array = np.array(features[1][0,:,:,:3])
feature_array = feature_array.reshape(1, 63,63,3)
max_pool = tf.keras.layers.MaxPooling2D(pool_size = 2, strides = 2)
model2 = tf.keras.models.Sequential([max_pool])
features_pooled = model2.predict(feature_array)
features_pooled = features_pooled.reshape(31,31,3)
```

```
vmin = np.min(features_pooled)
vmax = np.max(features_pooled)
for iFeatures in range(3):
    plt.figure()
    plt.imshow(features_pooled[:,:,iFeatures], vmin =0, vmax=vmax, cmap = 'gray')
    plt.xticks(np.array([0, 10, 20, 30]))
    plt.yticks(np.array([0, 10, 20, 30]))
```

The resulting figures are shown in Fig. S2.

## III. CNN TRAINING CODE

We provide a more extensive script in `CNN_Train_2D.py` to run the model training and save the result. The following example illustrates the main steps in the script and provides a minimal example to load data, generate and train the model.

```
# Load dependencies
from tensorflow.keras.preprocessing.image import ImageDataGenerator
import tensorflow as tf
import GStools as gst
import numpy as np
import pickle

# Load the required training and validation data
dataset_train = np.array(pickle.load(open("Dataset_2D_train.p", "rb")))
dataset_val = np.array(pickle.load(open("Dataset_2D_val.p", "rb")))
labels_train = pickle.load(open("Dataset_2D_train_label.p", "rb"))
labels_val = pickle.load(open("Dataset_2D_val_label.p", "rb"))

# Convert labels to integers and correct range
labels_train_int = gst.intLabels(labels_train)
labels_val_int = gst.intLabels(labels_val)

# Create augmented data generator. Note use of custom random scaling function
# from gst.
datagen_train = ImageDataGenerator(
    rotation_range=360,
    width_shift_range=1.0,
    height_shift_range=1.0,
    shear_range=0.2,
    zoom_range=0.2,
    horizontal_flip=True,
    preprocessing_function=gst.randscale,
```

```
    fill_mode="wrap",
    )
datagen_train.fit(dataset_train)

# Define the model
model = tf.keras.Sequential()
model.add(tf.keras.Input(shape=(128,128,3)))
model.add(tf.keras.layers.BatchNormalization())
model.add(tf.keras.layers.Conv2D(32, (3, 3), strides=2, activation="relu"))
model.add(tf.keras.layers.Conv2D(64, (3, 3), activation="relu"))
model.add(tf.keras.layers.MaxPooling2D(2, 2))
model.add(tf.keras.layers.Conv2D(128, (3, 3), activation="relu"))
model.add(tf.keras.layers.MaxPooling2D(2, 2))
model.add(tf.keras.layers.Conv2D(128, (3, 3), activation="relu"))
model.add(tf.keras.layers.MaxPooling2D(2, 2))
model.add(tf.keras.layers.GlobalMaxPooling2D())
model.add(tf.keras.layers.Dense(256, activation="relu"))
model.add(tf.keras.layers.Dropout(0.15))
model.add(tf.keras.layers.Dense(15))

# Compile model:
model.compile(
optimizer="adam", # this is a type of stochastic gradient descent
# Note that we need to set from_logits=True, because softmax is not explicitly
# set in last layer
loss=tf.keras.losses.SparseCategoricalCrossentropy(from_logits=True),
metrics=["sparse_categorical_accuracy"],
)

# Set batch size and number of epochs
Bsize = 128
Nepochs = 600
```

```
# Train the model:
history_training = model.fit(
datagen_train.flow(dataset_train, labels_train_int, batch_size=Bsize),
steps_per_epoch=len(dataset_train) / Bsize,
epochs=Nepochs,
validation_data=(dataset_val, labels_val_int),
)
```

## IV. SALIENCY MAPS

Unfortunately, as typical for neural networks, we do not get an intuitive picture of how the classification is performed. However, it is possible to determine which parts of the patterns activate the neural network particularly strong. For this we show so-called saliency maps, which highlight areas of images, which have been particularly important for the classification result. Different approaches to define such a quantity exist. We use a method based on the gradient of the classification accuracy with respect to small local changes of the input image. The intuitive interpretation of these maps is, that regions with a large gradient correspond to areas which are particularly important for the classification. We show these maps in Fig. S3c) for representative patterns from six classes. Notably, for many patterns, the model seems to be sensitive to very local features, such as the regions of activity, areas of transition or high and low concentrations.

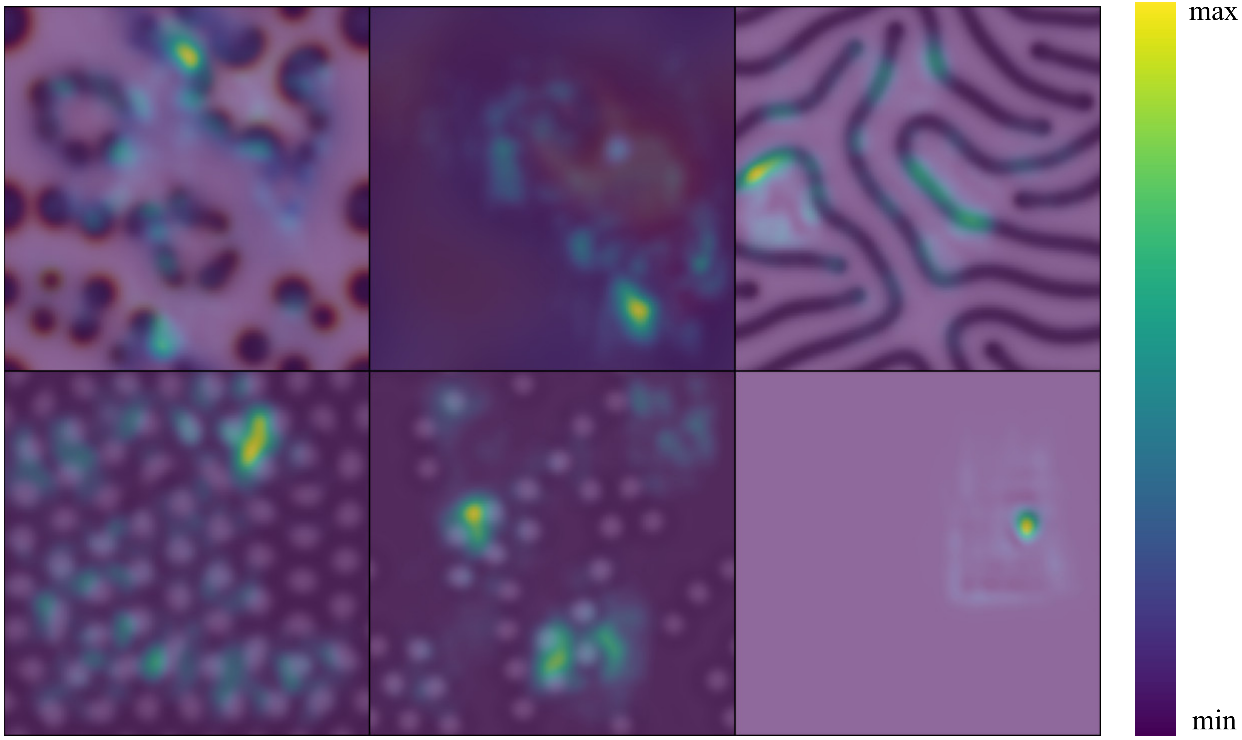


FIG. S3. Saliency maps for representative patterns drawn as overlays on representative patterns from different classes. The activation appears to be sensitive to local features of the patterns, such as areas of activity.

## V. SPATIAL AND TEMPORAL PROPERTIES OF PATTERNS

We can investigate if the model has correctly split homogeneous, heterogeneous and time-dependent patterns. We determine if a pattern is heterogeneous from its standard devaiation. If it is above a certain threshold, which can be obtained from the histogram across the entire scanned parameter space, we classify the pattern as heterogeneous (see red line in Fig. S4b). To determine if a pattern has significant time-dependence, we first calculate the 'velocity' $u(t+\Delta t)-u(t)$ and then calculate the root mean square of the resulting map. When this map is very different from zero we classify the pattern as time-dependent. Again we can determine a threshold for this intuitively from the histogram across the entire parameter space (see red line in Fig. S4c). Note that these thresholds are chosen based on human perception and in some cases the transition between patterns is gradual. However no qualitative differences are found for slight variations of the thresholds. We chart each class and determine whether the pattern belongs to a heterogeneous class and if it is time-dependent.

As shown in Fig. S4 we find that all patterns have been correctly associated with homogeneous and heterogeneous classes. Time-dependence appears to be in line with the semantic description of each phase, while in some classes only a fraction of patterns are time-dependent. These are classes where the final state is particularly sensitive to the initial conditions and finite system size.

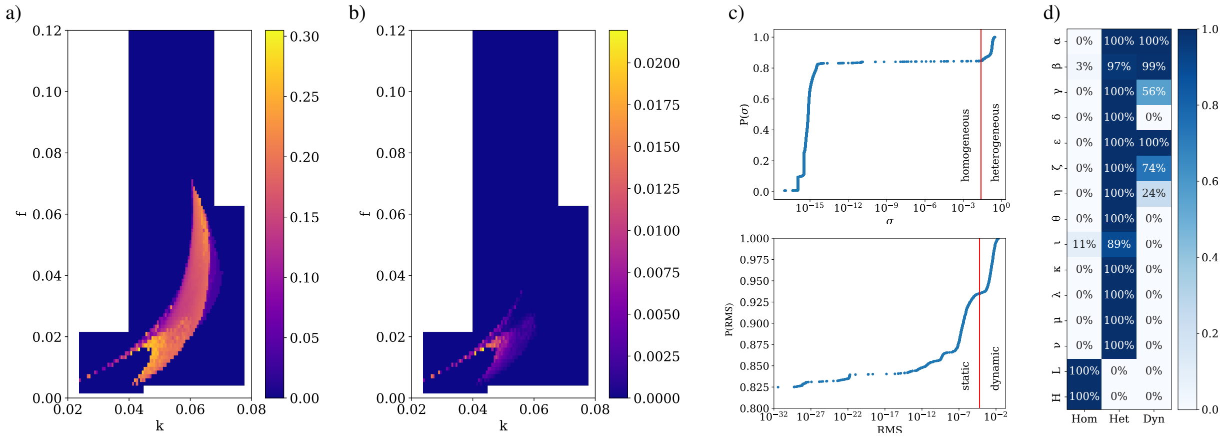


FIG. S4. a) Pattern standard deviation and parameter space dependence. A threshold to distinguish homogeneous from heterogeneous can be easily identified. b) RMS of the time-derivative of each pattern across the parameter space and the corresponding distribution. Again a threshold that distinguishes time-dependent from stationary patterns can be obtained from visual inspection. c) Cumulative distributions and thresholds (vertical lines) for $\sigma$ and RMS. d) Classifications of patterns cross-related to classes of homogeneous/heterogeneous and time-dependent patterns. The observation is inline with the semantic description of these patterns in the literature as discussed above.

## VI. 3D CONVOLUTIONAL NEURAL NETWORKS

For demonstration of an convolutional neural network with proper three-dimensional convolutions we use a time series of ten patterns $[u(t_1), ..., u(t_{10})]$ from a much longer time-frame, where $t_1 = 11400$, $t_2 = 11800$, ..., $t_{10} = 15000$, and combine these in a three-dimensional dataset, as illustrated in Fig. S5a). On this dataset, we can perform a three-dimensional convolution operation, which explicitly takes into account the possible correlations across different patterns in the timeseries. The architecture of the model is shown in Fig. S5b) and described in Table S1. The model is designed with fewer independent parameters compared to the 2D case, because the datasets for training are larger and the three-dimensional convolution is computationally more expensive. Hence, training takes a longer time.

In Fig. S6a) the training history of the optimization is illustrated. Again we approach a high accuracy of almost 96%, even though it is worse than the 2D model and fluctuations in the accuracy during training batches are more prominent. We evaluate our model with the training data and find a similar performance, as shown in the confusion matrix in Fig. S6b). In this case, training accuracy and test accuracy are very close to each other. In the test data we observe some misclassification between $\epsilon$, $\zeta$, $\eta$ and $\lambda$ resulting in a final accuracy of about 93%. Again these patterns share some similarities and transition between them could be gradual. In particular patterns with time-dependence can have long transitions where topologies of different classes overlap, which could explain the training accuracy fluctuations. However, in general, it appears that the three-dimensional model does not demonstrate con-

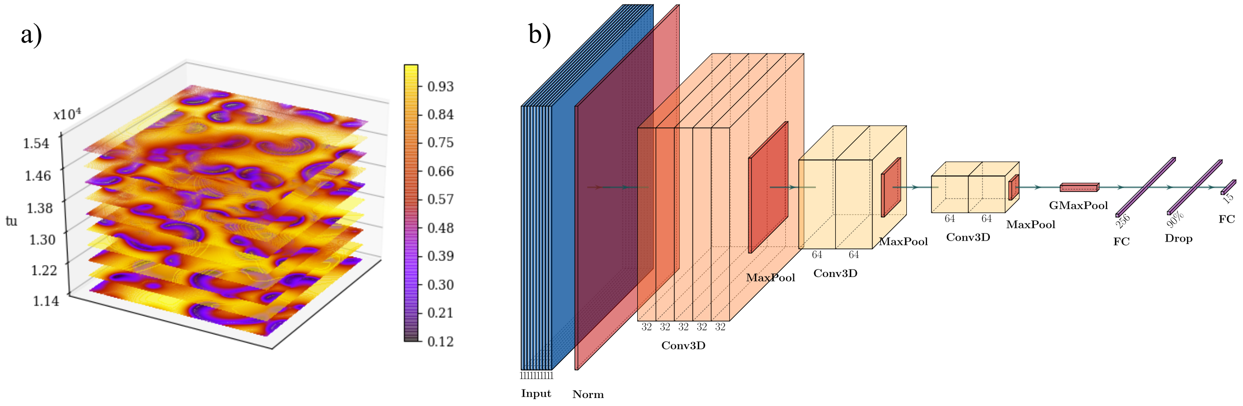


FIG. S5. a) Stack of ten patterns at different consecutive time-steps resulting in a 3D volumetric dataset per realization. b) Structure of neural network with layers and corresponding size.

TABLE S1. Architecture of 3D convolutional network. Layer type, size and strides of convolution kernel, activation function and number of parameters (fixed and trainable).

| Layer | Kernel | Output | Activation | Params. |
|---|---|---|---|---|
| Batch Norm. | - | 128, 128, 10, 1 | - | 4 |
| Conv3D | 3,3,2(2s) | 63, 63, 5, 32 | ReLU | 608 |
| MaxPool | 2,2,2 | 31, 31, 2, 32 | - | 0 |
| Conv3D | 3,3,1 | 29, 29, 2, 64 | ReLU | 18496 |
| MaxPool | 2,2,1 | 14, 14, 2, 64 | - | 0 |
| Conv3D | 3,3,1 | 12, 12, 2, 128 | ReLU | 36928 |
| MaxPool | 2,2,1 | 6, 6, 2, 128 | - | 0 |
| GlobMaxPool | - | 128 | - | 0 |
| Dense | - | 256 | ReLU | 16640 |
| Dropout | - | 256(90%) | - | 0 |
| Dense | - | 15 | softmax | 3855 |
| Total No. of Params. | | | | $\sum = 76531$ |

siderable advantages over the 2D-model. Computational cost, however, increases for 3D convolutions. For instance, training of the 3D model takes an order of magnitude longer than for 2D convolution features (this is partially due to a less efficient more high level python implementation). We concluded that we do not explicitly need to take temporal correlations into account in the convolutional layers and discuss results for the pure 2D convolution model in greater detail. There is a related method for classification of longer pattern sequences, such as videos, using convolutional neural networks. First, a CNN is used to transform each image in the sequence into the feature vector space and then perform a time-sequence classification on the resulting sequences, for instance using so-called recurrent neural networks. However, this is beyond the scope of this paper.

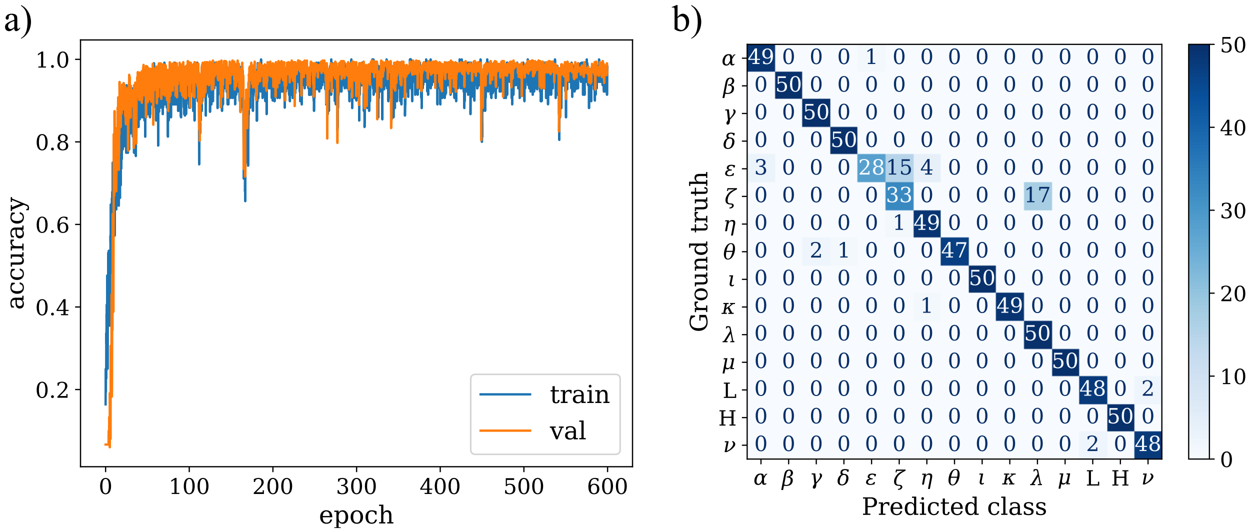


FIG. S6. a) Training history showing accuracy for training and validation data. The accuracy approaches 96% after about 600 epochs, however fluctuations during the training phase are noticably larger. b) Confusion matrix for the test dataset, depicting comparable results as in the 2D case with a total accuracy of about 93%.
